# Supplementary material for: Orbital engineering in nickelate heterostructures driven by anisotropic oxygen hybridization rather than orbital energy levels
Source: arXiv:1603.08873 ancillary file (2016-09-08)
Supplement: Supplementary file 1 [file Supplemental_Material.pdf]

# Supplemental Material for: Orbital engineering in nickelate heterostructures driven by anisotropic oxygen hybridization rather than orbital energy levels

G. Fabbri\*, D. Meyers, J. Okamoto, J. Pelliciari, A. S. Disa, Y. Huang, Z.-Y. Chen, W. B. Wu, C. T. Chen, S. Ismail-Beigi, C. H. Ahn, F. J. Walker, D. J. Huang, T. Schmitt, and M. P. M. Dean<sup>†</sup>  
(Dated: May 25, 2016)

This document provides further details and supporting measurements for the main manuscript. The experimental geometry for the resonant inelastic x-ray scattering (RIXS) measurements is depicted in Fig. S1. The high quality of the  $\text{LaTiO}_3 - \text{LaNiO}_3 - 3x(\text{LaAlO}_3)$  (LTNAO) and  $\text{LaNiO}_3$  films is demonstrated by x-ray reflectivity and surface diffraction measurements. A method for estimating crystal field parameters error bars is described. Ni  $L_3$  angular dependence, experimental and theoretical Ni  $L_2$  RIXS maps, as well as calculations using large  $\Delta e_g$  are used to corroborate the crystal field parameters described in the main text. Finally, the XAS spectra retrieved from the RIXS signal is compared to previous results to show that the present heterostructure also displays large orbital polarization.

## RIXS GEOMETRY

The experimental sample geometry is displayed in Fig. S1. Vertically ( $\sigma$ ) or horizontally ( $\pi$ ) polarized x-rays are incident at  $\theta_i$  on the sample, which has a  $c$ -axis surface normal. The incident x-ray electric field ( $\vec{e}$ ) is always parallel to  $b$  for  $\sigma$  polarization ( $b$  and  $a$  are equivalent by symmetry). On the other hand,  $\pi$  incident x-ray polarization probes a mixture of  $\vec{e} \parallel c$  and  $\vec{e} \parallel a$  contributions. Grazing x-ray incidence ( $\theta_i = 15^\circ$ ) is therefore used to maximize the  $\vec{e} \parallel c$  component in the  $\pi$  spectra. Note

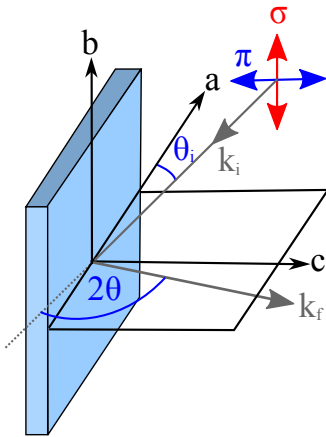

FIG. S1. (Color online) RIXS scattering geometry. Linearly polarized x-rays ( $\sigma$  or  $\pi$ ) are incident upon the sample at an angle  $\theta_i = 15^\circ$ . The scattered photons are collected at  $2\theta = 90^\circ$  and measured as a function of final energy.

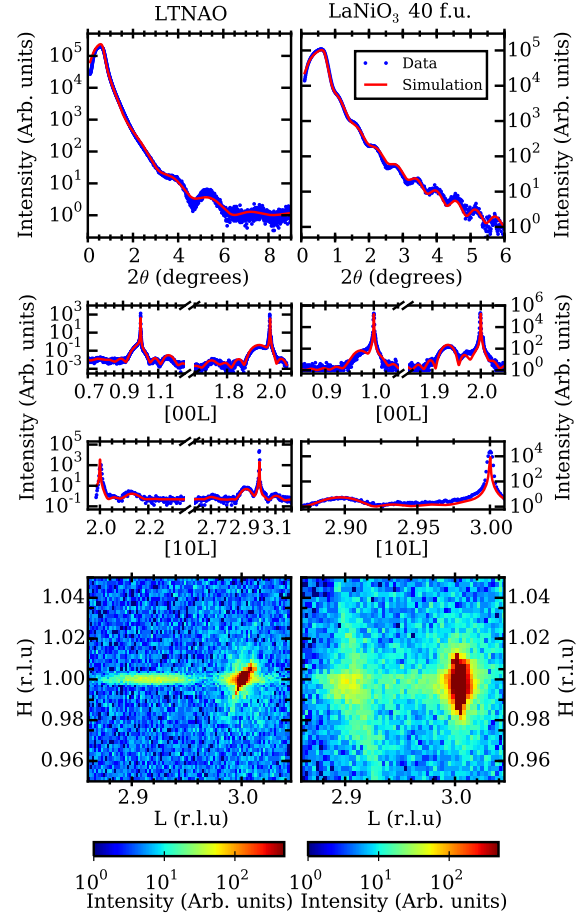

FIG. S2. (Color online) XRR and SXRD characterization of LTNAO (left) and  $\text{LaNiO}_3$  films (right). (Top) XRR (Middle) SXRD rods along  $[00L]$  and  $[10L]$ . (Bottom) 2d map of the  $(103)$  Bragg reflection, for both samples the  $ab$  plane is fully strained to the substrate.

that the  $\pi$  polarized simulated RIXS maps properly take into account this incident angle. The spectrometer is placed at  $2\theta = 90^\circ$  in order to minimize the Thompson scattering contribution to the  $\pi$  spectra.

## X-RAY REFLECTIVITY AND SURFACE DIFFRACTION

The structural quality of the LTNAO and  $\text{LaNiO}_3$  films used in this work was assessed using x-ray reflectivity

ity (XRR) and surface x-ray diffraction (SXRD). Measurements were performed in a Bruker D8 Discover machine equipped with a Cu  $K_\alpha$  x-ray source. The incident beam was vertically collimated using a Göbel mirror and monochromatized using a two bounce Ge (022) crystal. Slits of 0.1 mm (vertical) and 1 mm (horizontal) were used to define the beam size. The scattered beam was collected through a 0.5 mm detector slit and detected using a scintillator.

XRR and SXRD results are displayed in Fig. S2. Both films grew epitaxially to the  $\text{LaAlO}_3$  substrate. Simulations were performed using the GENX package [1]. The XRR reveals low surface roughness of  $5.2 \pm 0.3$  Å and  $3.3 \pm 0.4$  Å for LTNAO and  $\text{LaNiO}_3$  films, respectively. SXRD simulations were performed using the structure obtained on previous synchrotron-based SXRD study for LTNAO [2] and assuming a simple in-plane compressive strain for LNO. Despite the limitations imposed by the low flux of a Cu x-ray source (compared to a synchrotron), the excellent agreement between SXRD data and simulations and the small surface roughness obtained from XRR are strong evidences for the quality of the films used in this study. Further details of the sample preparation, including the oxygen growth conditions and oxygen annealing to avoid the formation of vacancies, can be found in the supplementary materials to Ref. 2.

### RIXS CALCULATIONS

This section provides further explanation of the RIXS calculations and computes the RIXS signal for different models in order to further confirm the results of the main text. In the approach used here, atomic wave functions are calculated via the Hartree-Fock method

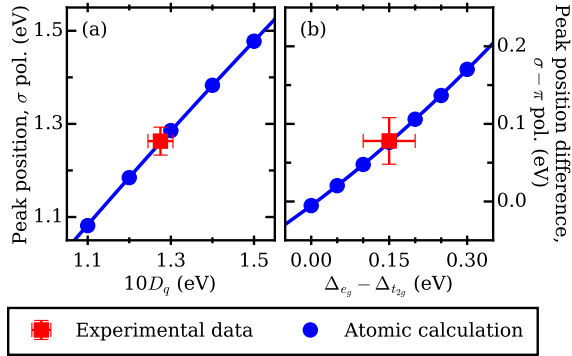

FIG. S3. (Color online) (a) Calculated position of the  $\sigma$  polarized RIXS main peak as a function of  $10D_q$ . The experimental measurement and error are consistent with  $10D_q = 1.28 \pm 0.03$  eV. (b) Difference between the RIXS main peak as measured by  $\pi$  and  $\sigma$  x-ray polarizations versus  $\Delta_{e_g} - \Delta_{t_{2g}}$ . Comparison with experimental value and error yields  $\Delta_{e_g} - \Delta_{t_{2g}} = 0.15 \pm 0.05$  eV.

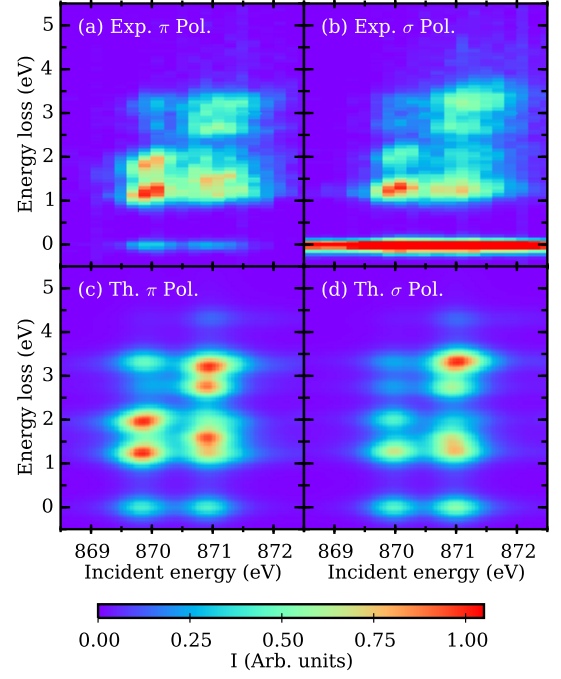

FIG. S4. (Color online) Color maps of the Ni  $L_2$  RIXS intensity of the LTNAO heterostructure. (a)&(b) plot the measured intensity with  $\pi$  and  $\sigma$  polarized incident x-rays. (c)&(d) plot the corresponding multiplet calculations for the two different polarizations.

using Cowan's codes [3]. Crystal fields are then introduced by mixing the atomic functions to generate the appropriate symmetry orbitals using Theo Thole's Racetrack code.  $L$ -edge RIXS involves two dipolar transitions via an intermediate state with a  $p$  core hole for example  $2p^6 3d^8 \rightarrow 2p^5 3d^9 \rightarrow 2p^6 3d^8 *$  where  $*$  denotes an orbital  $dd$ -transition [4]. The matrix elements for these transitions are calculated for dipole operators appropriate

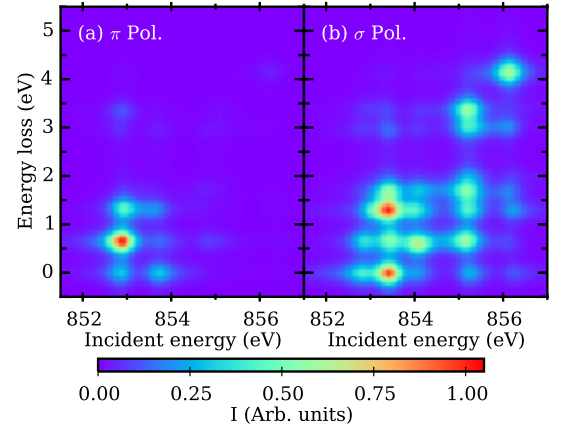

FIG. S5. (Color online) CTM calculation for Ni  $3d^8 L_3$  for  $\pi$  (a) and  $\sigma$  (b) polarization. The same parameters as shown in Table 1 of the main text were used, except  $\Delta_{e_g} = 0.8$  eV.

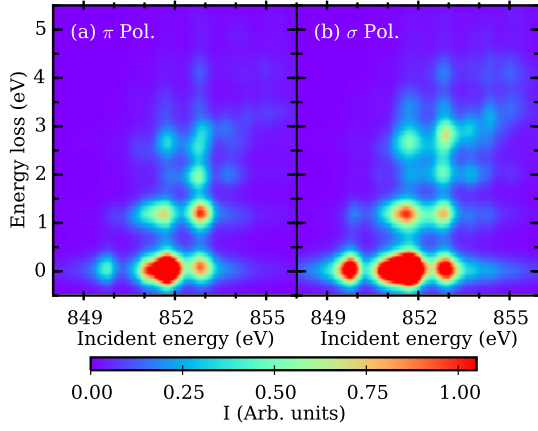

FIG. S6. (Color online) Atomic calculation for Ni  $3d^7 L_3$  for  $\pi$  (a) and  $\sigma$  (b) polarization. The same parameters as shown in Table 1 of the main text were used. Intensities were scaled to emphasize the inelastic features.

for the incident and final x-ray polarization and RIXS is then computed using the Kramers-Heisenberg equation. The effects of electron-electron interactions are incorporated using the Slater-Condon parameters.  $F_{dd}$  and  $F_{pd}$  set the percentage reductions in the Coulomb repulsion between two  $d$  electrons and  $p$ - $d$  electrons respectively [5].  $G_{pd}$  is the percentage reduction in the Coulomb exchange. The crystal field parameters  $10D_q$ ,  $\Delta t_{2g}$ , and  $\Delta e_g$  and the Slater-Condon parameters are determined semi-empirically via comparison between the calculation and the measurements. We note that each RIXS energy loss spectrum contains about four or more distinct spectral features (there are 35  $dd$  multiplets in the tetragonal symmetry). These features vary significantly for  $\sigma$  and  $\pi$  incident x-rays and resonate differently at two features in the Ni  $L_3$  XAS. Each feature is defined by an energy and an intensity. In this regard, there are a large number of spectral features, compared to the number of free parameters in the model, which justifies the use of such a procedure to find a unique solution. Only one overall intensity factor for each polarization is used to make the comparison between experiment and theory.

Error bars on the crystal field parameters were estimated using the energy loss of the main RIXS feature for both  $\pi$  and  $\sigma$  (Fig. 3(a)&(b) of the main text) using the following procedure. For  $\sigma$  polarization this feature's energy mostly depends on  $10D_q$ , i.e.  $E_\sigma \approx E_\sigma(10D_q)$ . This dependence is used to propagate the experimental error into  $10D_q$  (Fig. S3(a)). The same procedure is applied to the difference between  $\pi$  and  $\sigma$  polarized data, but in this case:  $E_\sigma - E_\pi \equiv \Delta E_{\sigma-\pi} \approx \Delta E_{\sigma-\pi}(\Delta e_g - \Delta t_{2g})$  (Fig. S3(b)). This leads to  $10D_q = 1.28 \pm 0.03$  eV and  $\Delta e_g - \Delta t_{2g} = 0.15 \pm 0.05$  eV. We note that this procedure likely overestimate the error bars by using only two features from the RIXS spectra. Therefore we estimate  $\Delta e_g = 0.2 \pm 0.05$  eV and  $\Delta t_{2g} = 0.05 \pm 0.05$  eV.

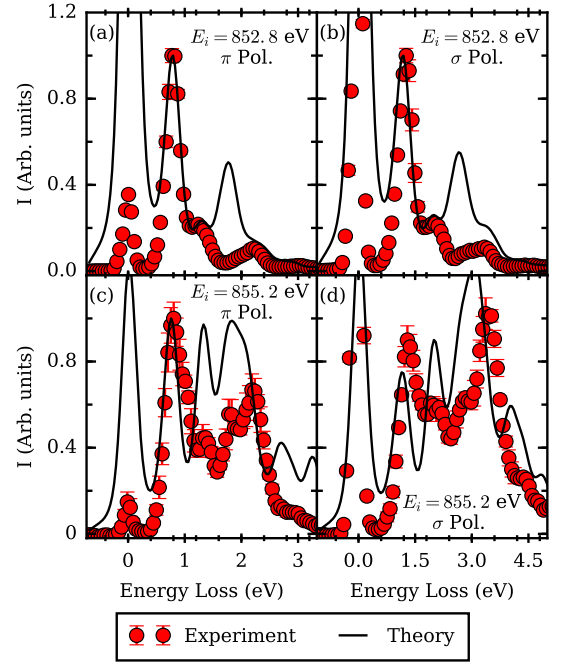

FIG. S7. (Color online) Line cuts of the atomic calculation for Ni  $3d^7 L_3$  are compared to the experimental data of LTNAO. (a)&(b) plot spectra at an incident energy of  $E_i = 852.8$  eV for  $\pi$  and  $\sigma$  polarized incident x-rays, respectively. (c)&(d) plot the same quantities for  $E_i = 855.2$  eV.

Several further tests were performed to confirm our modelling. Transition metal  $L$ -edge RIXS experiments are usually performed at the  $L_3$  ( $2p_{3/2}^4$  core state) edge in order to take advantage of its commonly larger cross section when compared to the  $L_2$  ( $2p_{1/2}^2$  core state). Nevertheless, here data was also collected at the Ni  $L_2$  edge of LTNAO to verify the results discussed in the main text. The data and atomic simulations are displayed in Fig. S4 using simulation parameters that are identical to those used for the Ni  $L_3$  edge. We find that the simulations are in excellent agreement with the experimental data, further demonstrating the robustness of the obtained crystal field parameters.

In order to exclude the presence of a very large  $e_g$  splitting we performed calculations with  $\Delta e_g = 0.8$  eV, but using the same values as shown in Table 1 for all other parameters. Figure S5 displays the calculated spectra demonstrating the inadequacy of such a model, which cannot be corrected by varying other parameters.

We also performed calculations assuming a Ni  $d^7$  state to test the possible validity of this configuration. Figs. S6 and S7 shows the calculated Ni  $L_3$  RIXS using the same crystal field parameters as in Table 1, revealing such a model is also incompatible with the measurements.

The small tetragonal crystal field acting upon Ni in LTNAO leads to similar RIXS spectra for  $\pi$  and  $\sigma$  x-ray polarizations collected at grazing incidence angle as

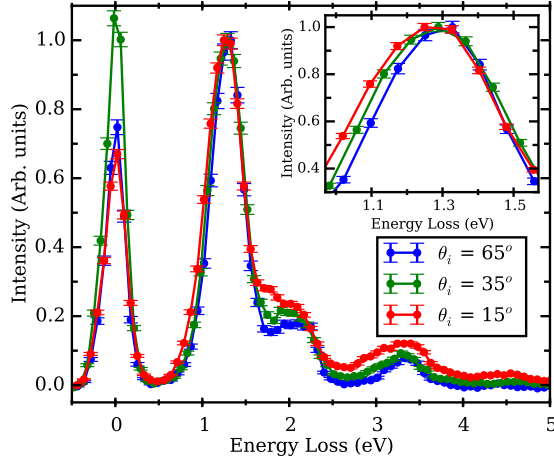

FIG. S8. (Color online) LTNAO Ni  $L_3$  edge RIXS as a function of incident angle. Data was collected at 853.8 eV incident energy and  $\pi$  polarization. A closer view of the main inelastic feature is displayed in the inset. A clear, small shift towards higher energy is observed with increasing angle.

shown in the main text. Such a lack of anisotropy can be alternatively verified by changing the incident x-ray angle while keeping the  $\pi$  polarization fixed. Fig. S8 displays the angular dependence of the LTNAO Ni  $L_3$  RIXS. The small shift of the main inelastic feature to higher energy loss with increasing angle is in agreement with the polarization dependence observed at grazing incidence, providing further evidence for a small Ni  $\Delta e_g$  splitting in LTNAO.

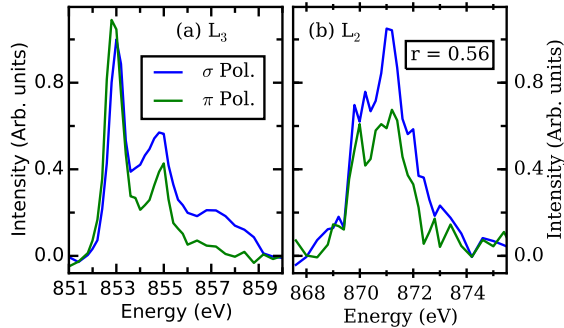

FIG. S9. (Color online) LTNAO Ni  $L_3$  (a) and  $L_2$  (b) Fluorescence yield XAS signal obtained by integrating the RIXS maps using energy loss larger than 0.5 eV. The hole ratio ( $r$ , see text for definition) extracted from  $L_2$  data agrees well with previously reported results [2], pointing to a strong orbital polarization in the Ni  $e_g$  states. The hole ratio is only marginally affected if the white line is included ( $r = 0.53$ ).

## X-RAY ABSORPTION SPECTROSCOPY

The x-ray fluorescence yield absorption spectroscopy spectra can be retrieved from the RIXS energy maps by integrating the intensities along the energy loss axis. This method was applied to the LTNAO Ni  $L_{2,3}$  RIXS and the results are displayed in Fig. S9. Integration was performed over energy loss greater than 0.5 eV, such cutoff was selected in order to remove the strong elastic contribution of La  $M_4$ , which peaks at  $\approx 850.5$  eV. The polarization dependence of the integrated XAS can be used to calculate the ratio of holes in the  $e_g$  orbitals [2, 6]:

$$r = \frac{h_{3z^2-r^2}}{h_{x^2-y^2}} = \frac{3I_z}{4I_{xy} - I_z} \quad (1)$$

where  $h_{3z^2-r^2}$  and  $h_{x^2-y^2}$  are the number of holes in each orbital, and  $I_{z,xy}$  is the integrated intensity for the incident x-ray polarization along  $z$  and  $xy$  plane. Note that  $r = 1/0$  for no/full orbital polarization. The hole ratio of 0.56 obtained from the RIXS data is in close agreement with that calculated from total fluorescence yield XAS in previous work on samples made through the same procedure [2].

\* gfabbri@bnl.gov

† mdean@bnl.gov

- [1] M. Björck and G. Andersson, J Appl. Cryst. **40**, 1174 (2007).
- [2] A. S. Disa, D. P. Kumah, A. Malashevich, H. Chen, D. A. Arena, E. D. Specht, S. Ismail-Beigi, F. J. Walker, and C. H. Ahn, Phys. Rev. Lett. **114**, 026801 (2015).
- [3] R. D. Cowan, *The Theory of Atomic Structure and Spectra* (University of California Press, Berkeley, 1981).
- [4] L. J. P. Ament, M. van Veenendaal, T. P. Devereaux, J. P. Hill, and J. van den Brink, Rev. Mod. Phys. **83**, 705 (2011).
- [5] F. De Groot and A. Kotani, *Core level spectroscopy of solids* (CRC press, 2008).
- [6] G. van der Laan, J. Phys. Soc. Japan **63**, 2393 (1994).
